# Supplementary material for: Rigorous Analysis of Software Countermeasures against Cache Attacks
Source: arXiv:1603.02187 source file (2017-05-11)
Supplement: Supplementary file 1 [file appendix.tex]

\clearpage
\section{Static Quantification of Leaks}\label{sec:quantleak}

In this section we characterize the amount of information leaked by a
program, and we show how this amount can be over-approximated by
static analysis. While the basic idea is standard, our presentation
differs from the literature in that we exhibit, at a high level of
abstraction, a new path for performing efficient quantitative
information-flow analysis while keeping low inputs symbolic. In
Sections~\ref{sec:statedom} and~\ref{sec:tracedom} we instantiate this
idea for the observers defined in Section~\ref{sec:security}.

\subsection{Quantifying Leaks}
As is common in quantitative information-flow analysis, we quantify the
degree of confidentiality provided by a program in terms of the
maximum number of observations an adversary can make, for any
valuation of the low input. Formally, we define leakage as
\begin{equation}\label{eq:leakage-low}
  \Leakage := \max_{\statelo\in\StatesInitLo}(\sizeof{\view(\collSemLo)})\ .
\end{equation}
This number comes with different interpretations in terms of security:
For example, it can be related to a lower bound on the expected number
of guesses an adversary has to make for successfully recovering the
secret input~\cite{massey94}, or to an upper bound for the probability of
successfully guessing the secret input in one
shot~\cite{smith09}.

\subsection{Static Bounds on Leaks, with Low Inputs}

For quantifying leakage based on Equation~\ref{eq:leakage-low}, one
needs to determine the size of the range of $\view$ applied to the
fixpoint $\collSemLo$ of the $\nextop$ operator, for all
$\statelo\in\StatesInitLo$ -- which is typically infeasible.

\gorancomment{Here it seems that two things are infeasible:
(1) fixpoint of $\collSem$; (2) doing this for all $\statelo$. Abstract 
interpretation is a solution for (1)}

For {\em fixed} values $\statelo\in \StatesInitLo$, however, the fixpoint
computation can be tractably approximated by abstract
interpretation~\cite{cousot:cousot77}. The result is a fixpoint
$\abs{\collSem}$ of the abstract transition function that represents a
superset of $\collSemLo$, based on which one can over-approximate the
range of $\view$~\cite{koepfrybal10}. This can be generalized to
arbitrary values of $\lambda$.
\gorancomment{Shouldn't we be talking about either $\collSem$ and
 $\abs{\collSem}$, or $\collSemLo$ and $\abs{\collSemLo}$?}

The novelty in this paper is that we compute fixpoints
$\abs{\collSem}(s)$ that contain dedicated symbols $s$ representing
the unknown value of the low input. The core advantage of using
symbols for representing low inputs (as opposed considering them to be
arbitrary values) is that it allows us to separate variations in
observable outputs due to low inputs (which are unproblematic) from
those that are due to high inputs (which consist potential leaks).

The semantics of $\abs{\collSem}(s)$ is given
with respect to a valuation $s\mapsto \lambda$ that instantiates $s$
with concrete value $\lambda\in\StatesInitLo$, and we denote it by
$\gamma_\statelo (\abs{\collSem}(s))$.\footnote{For simplicity of
  presentation we focus on one symbol and one low variable. In
  Section~\ref{sec:statedom} we use more general valuations.} With this
notation, we can express the {\em global soundness} of a symbolic fixpoint
as follows:
\begin{equation}\label{eq:globalsound}
\forall\statelo\in\StatesInitLo:
\collSem_\statelo\subseteq\gamma_\statelo\left( \abs{\collSem}(s) \right)
\end{equation}

Based on soundness of the symbolic fixpoint, we can immediately define
bounds for the leakage w.r.t. all low values.

\begin{equation}\label{eq:leakagebound}
 \Leakage \ \leq\ \max_{\statelo\in\StatesInitLo}
\sizeof{\view(\concSymb(\abs{\collSem}(s)))} 
\end{equation}
Even if we can compute an abstract fixpoint $\abs{\collSem}(s)$, the
right-hand side of Equation~\ref{eq:leakagebound} does not necessarily
lead to a practical algorithm for computing bounds on $\Leakage$
because it requires considering all concretizations
$\concSymb$. However, for abstract domains where the range of $\view$
can be computed based on the symbolic fixed point $\abs{\collSem}(s)$
alone, it can enable efficient computation of leakage bounds that hold
for all $\statelo\in\StatesInitLo$, as we show by example in
Section~\ref{sec:statedom}.

\section{Masked Symbol Abstract Domain}\label{sec:statedom}

Cache-aware code often uses Boolean and arithmetic operations on
pointers in order to achieve favorable memory alignment. In this
section we devise the \emph{masked symbol domain}, which is a simple abstract 
domain that enables the static
analysis of such code in the presence of dynamically allocated memory.

\subsection{Dynamic Memory as Low Data}
While dynamically allocated memory locations are not known in advance,
we make the simplifying assumption that the memory location returned
by \verb!malloc!  do not depend on secret data. More precisely, we
assume that those locations are part of the low initial state, i.e.,
$\StatesInitLo$ contains a pool of low heap locations that can
be dynamically requested by the program.

\begin{example}
  Consider a program that dynamically allocates heap memory for storing a secret
  key of size \verb!key_size! from a file \verb!key_file!.
\begin{verbatim}
         key = malloc(key_size);
         fread (key, 1, key_size, key_file);
\end{verbatim}
  If the key size is public, we consider the value of the pointer
  \verb!key! to be low, whereas the content of the region pointed
  to by \verb!key! is high.
\end{example}

%We capture low values by introducing \emph{symbolic values}, which are 
%assigned to each variable from $\StatesInitLo$. This allows distinguishing 
%between low and high values in adversaries' views: If a symbolic value is part 
%of the
%adversary's view, the adversary will observe the concrete 
%valuation of the value without learning additional information about the high 
%data. This results in a more precise counting of the adversary's observations.

\subsection{Representation}
The masked symbol domain is based on finite sets of what we call {\em
  masked symbols}, which are pairs $(\constsym,\mask)$ consisting of a
{\em symbol} $\constsym\in \Cons$ and a {\em mask}
$\mask \in\{0,1,\top\}^\bitlen$.  The idea is that the symbol $s$
represents an unknown base address and $\mask$ represents the pattern
of known and unknown bits. Here, $\{0,1\}$ stand for known bits and
$\top$ stands for unknown bits. The $i$-th bit of a masked symbol
$(\constsym,\mask)$ is hence equal to $\mask_i$, unless
$\mask_i=\top$, in which case it is unknown.In the first case we call
the bit {\em masked}, in the second {\em symbolic}. We abbreviate the
mask $(\top,\dots,\top)$ by $\top$.

Two special cases of masked symbols are worth pointing out:
\begin{compactenum}
\item $(\constsym,\top)$ represents an unknown constant, and
\item $(\constsym,\mask)$ with $\mask\in\{0,1\}^\bitlen$ represents the 
bit-vector $\mask$.
\end{compactenum}
That is, pairs of the form $(\constsym,\mask)$ generalize both bitvectors and 
unknown 
constants.

\subsection{Concretization and Counting}
We now give a semantics to elements of the masked symbol domain. This
semantics is parametrized w.r.t.\ instantiations of the symbols. For
the case where masked symbols represent partially known heap
addresses, a valuation corresponds to one specific layout.

Technically, we define the concretization of finite sets
$F\subseteq \Cons\times\{0,1,\top\}^\bitlen$ w.r.t.\ a mapping
$\symbmapping\colon \Cons\rightarrow \{0,1\}^\bitlen$ taking symbols to
bit-vectors:
\begin{equation*}
  \conc_\symbmapping(F)=\{\symbmapping(\constsym) \maskop \mask \mid 
(\constsym,\mask) \in F\} 
\end{equation*}
Here $\maskop$ is defined bitwise by $c_i\maskop m_i=m_i$ whenever
$m_i\in\{0,1\}$, and $c_i$ otherwise. Modeling $\lambda$ as a mapping
from symbols to bitvectors is a natural generalization of the
presentation in Section~\ref{sec:quantleak} to a low state consisting
of multiple components that are represented by different symbols.

\gorancomment{What is the exact difference between this 
$\symbmapping$ and the ``valuation'' from the previous section, and the 
connection to the $\lambda$ from the previous section?}

The following proposition shows that precise valuation of the constant
symbols can sometimes be ignored for deriving upper bounds on the
numbers of values that the novel domain represents. It enables the
quantification of information leaks in the absence of exact
information about locations on the heap.
\gorancomment{What does ``sometimes'' mean? I think it doesn't get clear that 
this is our approach for counting $F$.}

\begin{proposition}\label{prop:quant}
  For every valuation $\symbmapping\colon\Cons\rightarrow \{0,1\}^\bitlen$ and 
every
  projection $\view$ mapping vectors to a subset of their components, we have
  $\sizeof{\view(\conc_\symbmapping(F))}\le \sizeof{\view(F)}$
\end{proposition}
Proposition~\ref{prop:quant} gives us a means to derive upper bounds
on the range of the view of an adversary, for {\em any} valuation of
the symbols.
\begin{example}
  The projection of the set of (two bit) masked symbols
  \begin{equation*}
F=\{(s_1,(0,1)), (s_2,(\top,1)), (s_3,(1,1))\}
\end{equation*}
to their most significant bit yields the set $\{0,s_2,1\}$, i.e. we
count three observations. However, the projection to their least
significant bit yields only the singleton set $\{1\}$, i.e. the
observation is determined by the masks alone. We make use of this
observation for static reasoning about cache-aware memory alignment.
\end{example}
%Note that, so far we have not assumed any relationship between
%symbols. In Section we will increase the precision of our reasoning by
%tracking basic arithmetic relations between them.
%
\subsection{Update}
We support two kinds of operations on elements of the masked symbol
domain.  The first tracks patterns on bit-vectors and is needed for
reasoning about memory alignment. The second tracks the arithmetic
relationship between masked symbols and is needed for basic pointer
arithmetic and equality checks. Here we describe only operations
between pairs of masked symbols, the lifting of these operations to
sets of masked symbols is obtained by performing the operations on all
elements in their product.

\subsubsection{Tracking Bits}
An important class of operations for cache-aware coding are those that
allow the alignment of data to memory blocks without knowing the
precise pointer value.
\begin{example}\label{ex:maskop}
  The following code snippet allocates $1000$ bytes of heap memory and
  stores a pointer to this chunk in $x$. 
\begin{verbatim}
         x = malloc(1000); 
         y = (x & 0xFFFFFFC0) + 0x40;
\end{verbatim}
The second line ensures that the 6 least significant bits of that pointer are 
set to $0$, thereby aligning it with
  cache lines of $64$ bytes. Finally, adding \verb!0x40! ensures that the 
resulting pointer points into the allocated region while keeping the alignment. 
\end{example}
To reason about this kind of code, we distinguish between operations that allow 
the introduction of a mask and those that maintain a symbol: The left 
column of 
Table~\ref{tab:maskop} lists logical bit operations that translate symbolic 
bits 
into masked bits, i.e. creating a mask. For example, the operation 
\verb!x & 0xFFFFFFC0! in Example~\ref{ex:maskop} results in a masked symbol 
\begin{equation}\label{eq:lsbzero} 
(\constsym_x,(\top\cdots\top{}000000))\ .  
\end{equation}

\begin{table}
\begin{center} 
\begin{tabular}{|c|c|}\hline 
$s$ \verb! & ! $0=0$ & $s$ \verb! & ! $1=\top$\\
$s$ \verb! | ! $1=1$ & $s$ \verb! | ! $0=\top$\\
$s$ \verb! ^ ! $s=0$ & $s$ \verb! ^ ! $0 =\top$\\
$s$ \verb! - ! $s=0$ & \\ \hline
\end{tabular} 
\vspace{0.5em}
\caption{Bit operations and their effect on masked symbols. The 
left column shows operations that recover mask bits from symbols. The right 
column contains operations that leave symbolic bits 
unmodified.}\label{tab:maskop}
\end{center}
\end{table}

The right column in Table~\ref{tab:maskop} lists logical bit operations that 
leave symbolic bits unmodified, thus maintaining the symbol. Information about 
the mask can also be maintained throughout arithmetic operations such as 
additions, as long as all carry bits can be absorbed within the mask. For 
example, the addition of \verb!0x3F! to \eqref{eq:lsbzero} results in a masked
symbol 
\begin{equation*}
(\constsym_x,(\top\cdots\top{}111111))\ ,
\end{equation*}
for which we can statically determine containment in the same cache line as 
$(\constsym_x,(\top\cdots\top{}000000))$.

In cases when an operation $\circ$ does affect the symbolic bits, we take a 
conservative 
approach and drop information about the symbols. Formally,\begin{equation*}
(\constsym_1,\mask_1) \circ (\constsym_2,\mask_2) = (\constsym_3,\mask_3)\ ,
\end{equation*}
where $\constsym_3$ is a fresh symbol, and $\mask_3$ is determined according 
to Table~\ref{tab:maskop}. For example, the addition of \verb!0x40! 
to~\eqref{eq:lsbzero} in Example~\ref{ex:maskop} results in the masked symbol
\begin{equation*}
(\constsym_y,(\top\cdots\top{}000000))\ ,
\end{equation*}
which points to the beginning of some (unknown) cache line.

\subsubsection{Tracking Arithmetic Relationships}\label{ssec:arith_rel}
We add support for tracking basic arithmetic operations on masked
symbols, which is required to enable the analysis of low-level code.
\begin{example}\label{ex:pointers}
  The following code snippet computes the entries of array \verb!A!
  for indices $i=0,\dots,9$ using some function \verb!get_value!.
\begin{verbatim}
         int *x = A + 10;
         int *y;
         for (y = A; y < x; y++)
           *y = get_value (...);
\end{verbatim}
  The loop terminates whenever pointer \verb!y! points at or beyond
  \verb!x!. While comparisons on pointers can be avoided at the source
  level (using integer counters in the for condition), compilers often
  produce similar code patterns for efficiency.
\end{example}

The operations on symbols defined so far are not sufficient for a
precise analysis of the code in Example~\ref{ex:pointers}, e.g. in
case that \verb!A!  has a symbolic value $(s,\top)$. In this case, at
iteration $i = 2,3,4,\dots$ of the loop, the analysis will assign
\texttt{y} a fresh symbolic value $(s_i,\top)$. Without additional
knowledge, the equality or inequality between $s$ and $s_i$ cannot be
determined, which prohibits determining at which iteration the loop is
terminated.

To address this shortcoming, we
add support for tracking simple arithmetic congruences between
masked symbols. For masked symbols $s_1,s_2$, those congruences are terms
of the form $s_1 = s_2 + o$, where $o$ is an integer constant.
Building up a set of constraints $C$ between masked symbols allows establishing 
equalities between masked symbols. In the example above, at the first iteration 
of the loop we determine that $y = (s,\top)$ and $x = (s',\top) = (s,\top) + 
10$. After the tenth iteration of the loop, we determine that $y = (s',\top) = 
x$. 

Technically we track this relationship by maintaining a mapping of
type $\congrfn\colon\Cons\rightarrow(\Cons\times\{0,1\}^n)\cup{\bot}$
that stores, for every symbol, the symbol from which it was derived
together with the additive offset. Fresh symbols are assigned $\bot$.
We adapt the semantics $\conc_\symbmapping(F)$ of masked symbols to
account for such constraints by considering only symbol valuations
$\symbmapping\colon\Cons\rightarrow\{0,1\}^\bitlen$ that satisfy all
congruences, i.e.
\begin{equation*}
\symbmapping(s_1)\maskop m_1=\symbmapping(s_2)\maskop m_2 +o\ ,
\end{equation*} for all
$(s_1,m_1)=(s_2,m_2)+o \in F$.

\subsubsection{Tracking Flag Values}
Our analysis is performed at the level of disassembled x86 binary code, where 
inferring status flag values is crucial for precise reconstruction of the 
control flow. Returning to Example~\ref{ex:pointers}, the termination of the 
loop is established by the operation
\texttt{cmp~x,~y} followed by a conditional jump in case that the 
zero flag (\texttt{ZF}) is not set.

We support limited derivation of flag values for operations involving masked 
symbols. By default we safely assume no knowledge about flag values, and in 
the following cases we precisely determine flag values:
% 
% When performing an update involving masked symbols, control flag values may 
% be affected. By default we safely assume no knowledge about the flag values.  
% To 
% improve precision of the analysis, we identify several cases where flags are 
% determined even though values are symbolic. Among those cases, we identify 
% the 
% following:
\begin{compactenum}
 \item If at least one masked bit of the result is non-zero, then \texttt{ZF = 
0}.
 \item If the operation does not affect the (possibly symbolic) 
most-significant bits of the operands, then \texttt{CF = 0}.
\item \label{itm:midloop} For operation \texttt{sub src, dst} (or 
equivalently,
  \texttt{cmp src, dst}), if we can deduce that
  $\texttt{src} = \texttt{dst} + c$ with $c\neq 0$, then \texttt{ZF =
    0}.
\item \label{itm:endloop} For operation \texttt{sub src, dst} (or 
equivalently,
  \texttt{cmp src, dst}), if we can deduce that
  $\texttt{src} = \texttt{dst}$, then \texttt{ZF = 1}.
\end{compactenum}

% We apply the information learned about flags in combination with arithmetic 
% congruences, to establish loop termination.
% For example, at the end of the loop in Example~\ref{ex:pointers},  the 
% operation
% \texttt{cmp~x,~y} followed by a conditional jump determines the termination 
% of 
% the loop.

In Example~\ref{ex:pointers}, after loop iteration $i\in\{1,\dots,9\}$, 
case~\ref{itm:midloop} allows the analysis to establish that the conditional 
jump is 
taken, and that the loop is not terminated. At iteration $i=10$, the approach 
described in~\ref{ssec:arith_rel} establishes that \texttt{x = y}, and 
case~\ref{itm:endloop} allows the analysis to determine that the loop is 
terminated.

\subsection{Soundness}\label{ssec:soundness}
For establishing soundness of our analysis according to
Equation~\eqref{eq:globalsound}, we rely on a central result
from~\cite{cousot:cousot77} that states that \emph{local soundness}
implies global soundness. Here, we give a definition of local
soundness that is parametric in $\statelo$ to match our development.
\begin{equation}\label{eq:localsoundness}
  \forall\statelo\in\StatesInitLo, \forall a\in\abs{\Traces}:
\nextop\left(\concFTraces_\statelo(a)\right)\subseteq\concFTraces_\statelo(\abs{
    \nextop} (a))
\end{equation}
Local soundness states that the effect of each computation step is
overapproximated, in the sense that the computations reachable when
applying the abstract $\abs{\nextop}$-operator are a superset of the
computations reachable when applying the concrete $\nextop$-operator.

\begin{lemma}
 The masked symbol domain is locally sound.
\end{lemma}
Informally, the soundness follows from the soundness of the
ingredients of its update: (a) fresh symbols are introduced whenever
exact values are not known; (b) the trivial congruence $x = x + 0$ is
used whenever no congruence between $x$ and another masked symbol is
known; (c) all flag combinations are considered whenever the operation
does not determine the exact flags. We leave a formalization of this
argument to the extended version of this paper.~\TODO{This section is
  dissappointing.}
